# Supplementary material for: PatchIsland: Orchestration of LLM Agents for Continuous Vulnerability Repair
Source: arXiv:2601.17471 source file (2026-07-16)
Supplement: Supplementary file 1 [file claude_code.tex]

\begin{figure}[h]
    \centering
    \inputminted[breaklines,mathescape=false]{python}{code/claude_code.py}
    \caption{Example code for integrating \cc{Claude Code}. Parts not essential to the core logic are omitted; the full implementation is available in \repo.}
    \label{code:claude_code}
\end{figure}
